# Supplementary material for: Concept-aware clustering for decentralized deep learning under temporal shift
Source: arXiv:2306.12768 source file (2023-06-22)
Supplement: Supplementary file 2 [file info.tex]

4 Clusters,
all with same 8 labels.

In cluster 1 all images have "correct" labels
In cluster 2, two vehicle images have had their labels swapped
In cluster 3, two animal images have had their labels swapped
In cluster 4, two other animal images have had their labels swapped

10 time steps
200 rounds in each
20 clients
Random & Dac samples 6 clients per round -> HAST does 3 sampled on whole network, 3 sampled on aggregation layers
3 local training epochs

Clients follow cluster pattern in feddrift, i.e. initially all clients in cluster 1, over time they change back and forth ending up in a mix of different clusters

This test is on sentiment drift, $P^t(x) = P^{t+k}(x), P^t(y|x)\neq P^{t+k}(y|x)$, example someones preferences changes oven time

Through following a cluster pattern with unquealy many clients per cluster in each time step we also see a quantity drift, i.e. amount of data belonging to each cluster/distribution
