# Supplementary material for: Concept-aware clustering for decentralized deep learning under temporal shift
Source: arXiv:2306.12768 source file (2023-06-22)
Supplement: Supplementary file 3 [file info.tex]

4 Clusters,
all with same 8 labels.

In cluster 1 all images have "correct" labels
In cluster 2, two vehicle images have had their labels swapped
In cluster 3, two animal images have had their labels swapped
In cluster 4, two other animal images have had their labels swapped

10 time steps
200 rounds in each
50 clients
Random & Dac samples 6 clients per round -> HAST does 3 sampled on whole network, 3 sampled on aggregation layers
3 local epohcs, HAST does "6" as it trains whole network 3 epochs, finetunes part of network 3 epochs, but as seen in other figure, even when we doubled local epochs for DAC/random it was only detrimental for them

Clients follow random cluster pattern i.e. all clusters have equally many (as close as possible) clients in all time steps, but at each time step clients are assigned to a cluster through 1/(num clusters)

This test is on sentiment drift, $P^t(x) = P^{t+k}(x), P^t(y|x)\neq P^{t+k}(y|x)$, example someones preferences changes oven time
